# Supplementary material for: Transfer learning for scalability of neural-network quantum states
Source: arXiv:1908.09883 source file (2019-08-26)
Supplement: Supplementary file 1 [file appendix.tex]

\appendix
	\section{Choice of Parameters}
	\label{sec:param_expe}
	\dpc{No PBC but OBC.} 
	This section presents the empirical experiments and choice of parameters for the experimentation.
	We do all of the experiments on 64 particles of transverse field Ising model where the Hamiltonian parameters $h = J$. We stop the program when the dynamic stopping criterion explained in Section~\ref{sec:evaluation} is reached. There are four parameters in the training process that is need to be determined, namely the number of hidden nodes, the number of samples, choice of optimizer for gradient descent and the learning rate in the gradient descent.
	
	To determine the number of hidden nodes, we use the concept of density ($\alpha$) which is the ratio between the number of hidden nodes and visible nodes used in~\cite{carleo2017solving}.   Figure~\ref{fig:density} shows the result of the ground state energy and time with density values from $1$ to $10$. We see that the ground state energy and time drop significantly from density 1 to 2. However, if we keep increasing the density then the time grows faster than the reduction rate of the ground state energy. Carleo and Troyer~\cite{carleo2017solving} mentioned that the quality of the wave function improved with the size of the hidden nodes. However, from the figure, we see that we lose much on the efficiency than the effectiveness when we increase the density. Therefore, we set the density ($\alpha$) to be two because it is the most efficient.

        \begin{figure}[!htb]
            \centering
            \resizebox{0.5\textwidth}{!}{\input{figures/density.tex}}
            \caption {The ground state energy and time of $8\times 8$ particles of Transverse Field Ising (TFI) model with Periodic Boundary Conditions (PBC) with different density (ratio of hidden nodes and visible nodes) after trained to the dynamic stopping criterion.}    
                  \label{fig:density}
                
        \end{figure}

        Figure~\ref{fig:samples} shows the result of the ground state energy and time with number of samples from $1000$ to $100,000$. Similar to the density experiments, we see that the ground state energy drop after $10,000$ samples and plateaued after that while the time grows exponentially. Therefore, we set the number of samples to be $10,000$ with the similar reason as the density experiments.
        
        \begin{figure}[!htb]
            \centering
    
            \resizebox{0.5\textwidth}{!}{\input{figures/num_samples.tex}}
            \caption
            {The ground state energy and time of $8\times 8$ particles of Transverse Field Ising (TFI) model with Periodic Boundary Conditions (PBC) with different number of samples after trained to the dynamic stopping criterion.}      
            \label{fig:samples}
            
        \end{figure}
        
        We try five optimizers for the gradient descent algorithm available on the Tensorflow~\cite{abadi2016tensorflow} library namely vanilla Gradient Descent without optimizer, Adadelta~\cite{zeiler2012adadelta}, RMSProp~\cite{hinton2012neural}, Adam~\cite{kingma2014adam} and Adagrad~\cite{duchi2011adaptive} with its default parameters. Figure~\ref{fig:optimizer} shows the ground state energy and time for different optimizer. We see that Adam gives the lowest ground state energy and the fastest one. Therefore, we choose Adam as our optimizer. We see that the default learning rate for Adam which is $0.001$ does not converge for system with large scale such as $16\times 16$ and $8\times 8 \times 8$. For those two cases, we set the learning rate to $0.0001$.
        
        \begin{figure}[htb]
            \centering
            \begin{subfigure}[b]{0.475\textwidth}
                \centering
                 \resizebox{\textwidth}{!}{\input{figures/optimizer-energy.tex}}
                \caption[Network2]%
                {The energy with different optimizer.}    
                \label{fig:base}
            \end{subfigure}
            \hfill
            \begin{subfigure}[b]{0.475\textwidth}  
                \centering 
                \resizebox{\textwidth}{!}{\input{figures/optimizer-time.tex}}
                \caption[]%
                {The time with different optimizer.}    
                \label{fig:random}
            \end{subfigure}    
            \caption[]%
            {The ground state energy and time of $8\times 8$ particles of Transverse Field Ising (TFI) model with Periodic Boundary Conditions (PBC) with different optimizer after trained to the dynamic stopping criterion.} 
            \label{fig:optimizer}
        \end{figure}

    %   \begin{figure*}[!htb]
    %         \centering
    
    %         \resizebox{\textwidth}{!}{\input{figures/optimizer-energy.tex}}
    %         \caption[Network2]%
    %         {Parameters of the base network.}    
    %         \label{fig:base}
            
    %     \end{figure*}

    %   \begin{figure*}[!htb]
    %         \centering
    
    %         \resizebox{\textwidth}{!}{\input{figures/optimizer-time.tex}}
    %         \caption[Network2]%
    %         {Parameters of the base network.}    
    %         \label{fig:base}
            
    %     \end{figure*}
